# Supplementary material for: Structure Before Intelligence: Gating What Agentic Scientific Workflows Release
Source: arXiv:2610.19507 source file (2026-10-14)
Supplement: Supplementary file 2 [file supplement_arxiv.tex]

\def\arxivbuild{1}
\input{supplement}
